# Supplementary material for: Crabs: Consuming Resource via Auto-generation for LLM-DoS Attack under Black-box Settings
Source: arXiv:2412.13879 source file (2025-05-26)
Supplement: Supplementary file 1 [file appendix_Qwen_Q-num.tex]

\begin{table}[t]
\centering
\resizebox{\columnwidth}{!}{%
\begin{tabular}{@{}c|c|c|c|c|c@{}}
\toprule
\textbf{} & \textbf{1} & \textbf{2} & \textbf{4} & \textbf{8} & \textbf{16} \\ \midrule
\textbf{Typical Requests} & 40.5 & 40.5 & 45.5 & 46 & 50.5 \\
\textbf{AutoDoS}          & 47   & 48.5 & 49.5 & 51.5 & 50.5 \\ \bottomrule
\end{tabular}%
}
\caption{When allocating 50\% of GPU resources, different numbers of concurrent requests are executed on the Qwen model. This table compares the resource consumption differences between AutoDoS and typical requests.}
\label{tab:Qwen-Q-num}
\end{table}
